# Supplementary material for: SCORES: Shape Composition with Recursive Substructure Priors
Source: arXiv:1809.05398 source file (2018-09-14)
Supplement: Supplementary file 1 [file appendix.tex]

\begin{appendices}

\small

\section{Convergence analysis}
\label{apd:convergence}

The convergence of our iterative algorithm can be explained by the fact that both steps in each iteration decrease the optimization objective. {\em First}, the hierarchy inference ensures that the overall representation error does not increase, due to the schemes of error-minimizing sampling and non-error-increasing updating of hierarchies. {\em Second}, let us consider the local adjustment step for geometric deformation and full synthesis separately. For each substructure, geometric adjustment decreases the representation error by ``snapping'' the outer code at the root of the substructure to the nearest entry in the discrete latent space. The explanation of how re-synthesis decreases the objective is not as direct. In fact, the synthesis networks are trained to denoise the same set of substructures used for learning the discrete latent space of substructures (see the next section for details). Thus, given a substructure, it strives to generate a new one which is more similar to the ``seen'' ones from the training set. Since any training substructure has a low representation error by definition, the generation implicitly decreases representation error. Taken together, these factors induce convergence.

\section{Training and testing details}
\label{apd:details}

\mypara{Training.}
The training is split into three parts: for the substructure model (the codebook) and for the two denoising networks for local adjustment and re-synthesis, respectively. Note, however, that the latter two networks share the encoding component. Also, the codebook for the substructure model and for the local adjustment network can be jointly learned, since the former depends on the inner encoding and outer decoding of the latter.

The substructure model is trained based on pre-existing hierarchies of training shapes, computed by applying GRASS~\cite{li2017}. Each internal node in a hierarchy then contributes a valid substructure which can be used as a training example, for which the VQ representation loss is minimized. The reconstruction error for all boxes is minimized simultaneously. Thus, given an OBB structure $\cB$ with its associated hierarchy $\cH$, the overall training loss is:
\begin{equation}\label{eq:fgloss}
%  L & = L_\text{recon} + L_\text{VQ} \nonumber \\
%  & = \sum_{b\in \cB} \left\| f_\text{dec}^\text{out}(f_\text{enc}(\cB,\cH))|_b - b \right\| +
%  \sum_{n\in \cH} \left\| z_q(f_\text{enc}(S_n)) - f_\text{enc}(S_n) \right\|, \nonumber \\
  L = \underbrace{\sum_{b\in \cB} \left\| f_\text{dec}^\text{box}(x_b^\text{in},x_b^\text{out}) - b \right\|_2^2}_\text{recon. loss} + \underbrace{\sum_{n\in \cH} \left\| z_q(x_n^\text{out}) - x_n^\text{out} \right\|_2^2}_\text{VQ loss},
\end{equation}
%\begin{equation}\label{eq:smloss}
%  \sum_{b\in \cB} \left\| f_\text{dec}^\text{out}(f_\text{enc}(\cB,\cH))|_b - b \right\| \ + \ \sum_{n\in \cH} \left\| z_q(f_\text{enc}(S_n)) - f_\text{enc}(S_n) \right\|,
%\end{equation}
where $f_\text{dec}^\text{box}$ is the box decoder. The training process involves tuning both the encoder and decoder networks, and the learning of the codebook for the discrete latent space. The latter is conducted in a manner similar to van den Oord et al.~\shortcite{oord2017}. Figure~\ref{fig:trainadjust} shows the training process.

\begin{figure}[t!] \centering
	\begin{overpic}[width=1.0\linewidth,tics=10]{train_adjust}%,grid
    %\put(18,5){\small (a)}
    %\put(59,-3){\small (b)}
    %\put(85,-3){\small (c)}
	\end{overpic}
    \caption{Joint training of substructure model (latent space dictionary learning) and geometric adjustment model (denoising network training). Two losses, VQ representation loss and OBB-wise self-reconstruction loss, are minimized. The network connections for bottom-up encoding and top-down decoding are simplified into grey double arrows, for clarity.}
    \label{fig:trainadjust}
    \vspace{-7pt}
\end{figure}

Training the substructure codebook implicitly also yields a local adjustment mechanism. This is because the trained outer code decoder has the effect of denoising when its input code is `snapped' to the nearest entry in the discrete latent space. Therefore the encoder, codebook and outer decoder jointly constitute the local adjustment framework during testing (see below).

To train a GRASS-type network for re-synthesis of substructures where the representation error is too large, we create noisy/clean substructure pairs by perturbing training shapes. To make the network robust to different inferred hierarchies, we generate several different encoding hierarchies for the same training shape, through randomly altering the original one. For each internal node of a given hierarchy and its corresponding subtree, we conduct the following perturbations:
\begin{enumerate}
\item Randomly perturb the position, scale, and orientation of all OBBs.
\item Randomly remove up to $20\%$ of the OBBs and rebuild a subtree for the remaining OBBs.
\item Randomly duplicate up to $20\%$ of the OBBs and rebuild a subtree for the new set of OBBs.
\end{enumerate}
All perturbations are via Gaussian noise. The maximum noise amplitude is $10\%$ of the bounding box diagonal of the entire shape for part position, $80\% \sim 120\%$ of the part OBB for scaling, and $\pm 10^\circ$ for orientation. For part removal, the new hierarchy is constructed by path collapse of the original one. For part duplication, on the other hand, a new hierarchy is built from scratch, in a greedy manner similar to GRASS.

The training loss for substructure re-synthesis is defined at each internal node, comprising a reconstruction loss (to generate clean output that is similar to the training input before perturbation) based on its inner code, and a node classification loss for determining the type (adjacency, symmetry, or leaf) of a generated node as in GRASS. The reconstruction loss can be written as:
\begin{equation}\label{eq:fgloss}
  \sum_{n \in \cH} \sum_{b \in \cB} \left\| F_\text{dec}^\text{gen}(F_\text{enc}(\tilde{\cB}(S_n),\tilde{\cH}(S_n)),b) - b \right\|_2^2,
\end{equation}
where $F_\text{dec}^\text{gen}(F_\text{enc}(\tilde{\cB}(S_n),\tilde{\cH}(S_n)),b)$ represents the bottom-up encoding of the substructure $S_n$ followed by a top-down decoding reaching a leaf node $b$. $\tilde{\cB}(S_n)$ and $\tilde{\cH}(S_n)$ denote the perturbed OBBs and hierarchy for substructure $S_n$. Figure~\ref{fig:traingen} shows the training process.

\begin{figure}[t!] \centering
	\begin{overpic}[width=1.0\linewidth,tics=10]{train_gen}%,grid
    %\put(18,5){\small (a)}
    %\put(59,-3){\small (b)}
    %\put(85,-3){\small (c)}
	\end{overpic}
    \caption{Training of synthesis model with the substructure corresponding to the internal node shaded in red. Since this model shares the encoder with the geometric adjustment model, it simply clones and fine-tunes the decoder trained by the latter. The training minimizes OBB-wise self-reconstruction loss.}
    \label{fig:traingen}
    \vspace{-7pt}
\end{figure}

\mypara{Testing.}
We now describe the testing of the trained models for hierarchy inference and local adjustment. During hierarchy inference, the evaluation of a newly sampled hierarchy involves applying the substructure model to compute VQ representation error. Then, given a sampled hierarchy, we first perform a bottom-up encoding of the current set of OBBs using the encoder network $f_\text{enc}$. We then use $f_\text{dec}^\text{out}$ to compute an outer code for each internal node (not including root or leaf nodes) in a top-down pass. The VQ representation error for an internal node is then computed based on its outer code, using Equation (5) in the main paper.

Once a hierarchy is inferred, we first perform a bottom-up encoding to compute the inner code for each node. The local adjustment is performed in a top-down cascade fashion. Starting from the highest-level node, we perform the following steps for each internal node. We first compute its outer code and use this to estimate its VQ representation error. If the error, combined  with a factor penalizing node depth to yield the metric $\eta(S_n)$, is smaller than the user-prescribed threshold $\eta_\text{T}$, then outer decoding is performed for its children recursively. When the metric exceeds the threshold, full re-synthesis is launched at this node. When the top-down decoding reaches a leaf node, the box decoder is invoked to reconstruct the output OBB parameters from both inner and outer codes.

\mypara{Hyperparameters.}
Inner and outer codes are $80$-dimensional. The layer sizes of the MLPs are as follows:
\begin{itemize}
  \item {\em Inner code encoder.} $2 \times 80 = 160$ (two children) or $80 + 8 = 88$ (symmetry group) for input layer, $200$ for each of two hidden layers, $80$ for output layer (parent code).
  \item {\em Outer code decoder.} $2 \times 80 = 160$ for input layer (parent and sibling inputs), $200$ for each of two hidden layers, $2 \times 80 = 160$ (two children) or $80 + 8 = 88$ (symmetry group) for output layer.
  \item {\em Box encoder.} $12$ for input layer (OBB parameters), $200$ for each of two hidden layers, $80$ for output layer (leaf inner code).
  \item {\em Box decoder.} $2 \times 80 = 160$ for input layer (leaf inner and outer codes), $200$ for each of two hidden layers, $12$ for output layer (OBB parameters).
\end{itemize}
The code definition for box ($12$D) and symmetry ($8$D) parameters is the same as GRASS~\cite{li2017}.
The size of the codebook for the discrete latent space is $2048$, with a dimension of $8$.
The training adopts ADAM optimization, with a batch size of $50$.
We employ multi-step learning rate scheduling, which sets the initial learning rate to $1\times 10^{-4}$,
and decays it to $1\times 10^{-4}$ at epoch $100$, and to $1\times 10^{-6}$ at epoch $500$.

\end{appendices}
